# Supplementary material for: SoK: Critical Evaluation of Quantum Machine Learning for Adversarial Robustness
Source: arXiv:2511.14989 source file (2026-05-21)
Supplement: Supplementary file 1 [file Huang_noisy.tex]

% ============================================================
% TABLE 2: Noisy (Depolarizing p=0.01) CA and ASR
% ============================================================
\begin{table}[!t]
\caption{Huang Backdoor Attack: Clean Accuracy (CA\%) and Attack Success Rate (ASR\%) under Depolarizing Noise ($p=0.01$).}
\label{tab:huang_noisy}
\centering
\scriptsize
\setlength{\tabcolsep}{4pt}
\begin{tabular}{@{}c|c|c|cc|cc@{}}
\toprule
\multirow{2}{*}{\textbf{Enc.}} & \multirow{2}{*}{\textbf{Layer}} & \multirow{2}{*}{{\shortstack{\textbf{Poison}\\\textbf{Ratio}}}} & \multicolumn{2}{c|}{\textbf{AZ-Class}} & \multicolumn{2}{c}{\textbf{MNIST}} \\
\cmidrule(lr){4-5} \cmidrule(l){6-7}
& & & \textbf{CA (\%)} & \textbf{ASR (\%)} & \textbf{CA (\%)} & \textbf{ASR (\%)} \\
\midrule
\multirow{9}{*}{\rotatebox[origin=c]{90}{\textbf{Amplitude}}}
& \multirow{3}{*}{2}
  & 0.1 & 34.59$\pm$1.07 & 71.93$\pm$4.55 & 44.85$\pm$2.43 & 28.05$\pm$2.66 \\
& & 0.3 & 34.41$\pm$1.44 & 100.00$\pm$0.00 & 44.34$\pm$2.74 & 100.00$\pm$0.00 \\
& & 0.5 & 33.41$\pm$1.95 & 100.00$\pm$0.00 & 42.98$\pm$2.77 & 100.00$\pm$0.00 \\
\cmidrule(lr){2-7}
& \multirow{3}{*}{10}
  & 0.1 & 23.52$\pm$1.88 & 28.84$\pm$4.22 & 35.01$\pm$ 2.17 & 32.33$\pm$3.34 \\
& & 0.3 & 23.54$\pm$1.81 & 96.39$\pm$2.11 & 35.77$\pm$2.21 & 95.72$\pm$2.48 \\
& & 0.5 & 22.80$\pm$2.16 & 99.75$\pm$0.04 & 35.78$\pm$2.54 & 98.55$\pm$1.01\\
\cmidrule(lr){2-7}
& \multirow{3}{*}{50}
  & 0.1 & 4.35$\pm$2.46 & 2.58$\pm$1.88 & 6.44$\pm$2.47 & 7.88$\pm$3.52 \\
& & 0.3 & 5.36$\pm$3.44 & 4.39$\pm$1.02 & 7.38$\pm$3.37& 6.94$\pm$3.65 \\
& & 0.5 & 5.78$\pm$3.79 & 5.50$\pm$2.55 & 7.59$\pm$3.21& 7.06$\pm$2.92\\
\midrule
\multirow{9}{*}{\rotatebox[origin=c]{90}{\textbf{Angle}}}
& \multirow{3}{*}{2}
  & 0.1 & 45.27$\pm$1.99 & 0.48$\pm$0.33  & 48.80$\pm$2.23 & 91.40$\pm$2.92 \\
& & 0.3 & 44.81$\pm$2.00 & 28.80$\pm$1.88 & 48.54$\pm$4.33 & 93.97$\pm$1.93 \\
& & 0.5 & 44.86$\pm$1.68 & 55.90$\pm$1.48 & 43.88$\pm$2.39 & 96.39$\pm$2.82 \\
\cmidrule(lr){2-7}
& \multirow{3}{*}{5}
  & 0.1 & 47.32$\pm$1.22 & 2.29$\pm$1.02  & 52.10$\pm$2.33 & 80.55$\pm$2.56 \\
& & 0.3 & 48.07$\pm$1.64 & 16.88$\pm$3.22 &50.94$\pm$2.98 & 92.03$\pm$2.41 \\
& & 0.5 & 47.49$\pm$1.47 & 50.28$\pm$3.46 & 52.53$\pm$2.17 & 91.16$\pm$2.43 \\
\cmidrule(lr){2-7}
& \multirow{3}{*}{10}
  & 0.1 & 41.27$\pm$1.51 & 1.26$\pm$0.76  & 49.16$\pm$1.99 & 51.64$\pm$2.99 \\
& & 0.3 & 41.53$\pm$1.15 & 2.38$\pm$1.12  & 49.36$\pm$2.03 & 53.08$\pm$2.72 \\
& & 0.5 & 41.70$\pm$2.38 & 4.10$\pm$1.57  & 39.57$\pm$2.60 & 60.10$\pm$2.35 \\
\bottomrule
\end{tabular}
\end{table}
